# Supplementary material for: Strong Byzantine Agreement with Adaptive Word Complexity
Source: arXiv:2308.03524 source file (2023-08-07)
Supplement: Supplementary file 1 [file proof_transformation.tex]

\section{\name: Formal Proof of Correctness \& Complexity}

In this section, we prove the correctness and complexity of \name (\Cref{algorithm:strong_new}).
Recall that, in \name, there are three types of certificates:
\begin{compactenum}
    \item Fast certificates: These certificates are obtained in \cert; correct processes obtain fast certificates at line~\ref{line:fast_certificate_obtained}.
    
    \item Specific certificates:
    We say that a certificate $\Sigma_v$ is a \emph{specific} certificate for a value $v$ if and only if $\Sigma_v$ is a (combined) threshold signature such that $\mathit{CombinedVerify}^{t + 1}(v, \Sigma_v) = \mathit{true}$.
    Correct processes obtain specific certificates at line~\ref{line:obtain_specific_certificate}.
    
    \item General certificates:
    We say that a certificate $\Sigma_g$ is a \emph{general} certificate if and only if $\Sigma_g$ is a (combined) threshold signature such that $\mathit{CombinedVerify}^{t + 1}(\text{``any value''}, \Sigma_g) = \mathit{true}$.
    Correct processes obtain general certificates at line~\ref{line:obtain_general_certificate}.
\end{compactenum}
Importantly, any certificate contains only $O(1)$ signatures.

\paragraph{Proof of correctness.}
First, we prove that \name satisfies strong validity.
To this end, we show that, if all correct processes propose the same value, then every correct process obtains a certificate by round 3.

\begin{lemma} \label{lemma:by_round_3}
If all correct processes propose the same value, then every correct process obtains a certificate by the beginning of round 3.
\end{lemma}
\begin{proof}
Let all correct processes propose the same value $v$.
We distinguish two possible cases:
\begin{compactitem}
    \item Let there exist a correct process which obtains a fast certificate before round 1 (at line~\ref{line:fast_certificate_obtained}).
    In this case, every correct process obtains a certificate by the beginning of round 3.
    Thus, the statement of the lemma holds in this scenario.
    
    \item Let no correct process obtain a fast certificate before round 1.
    In this case, every correct process broadcasts a \textsc{help\_req} message (line~\ref{line:broadcast_help_req}).
    Thus, every correct process receives \textsc{help\_reply} messages from all other correct processes, which implies that every correct process receives (at least) $t + 1$ partial signatures of $v$ at the beginning of round 3 (at line~\ref{check_for_broadcast_final_certificate}).
    Hence, every correct process obtains a certificate by the beginning of round 3.
\end{compactitem}
As in both possible cases the statement of the lemma holds, the proof is concluded.
\end{proof}

Finally, we are ready to prove that \name satisfies strong validity.

\begin{lemma} \label{lemma:strong_validity}
\name (\Cref{algorithm:strong_new}) satisfies strong validity.
\end{lemma}
\begin{proof}
By contradiction, suppose that all correct processes propose the same value $v$, and a correct process decides some value $v' \neq v$ (at line~\ref{line:decide_strong}).
Thus, there exists a certificate $\Sigma'$ for $v'$.
Let us consider all possible cases:
\begin{compactitem}
    \item Let $\Sigma'$ be a fast certificate.
    However, the existence of $\Sigma'$ is impossible due to the safety property of \textsc{bucket}.
    Thus, this case is impossible.
    
    \item Let $\Sigma'$ be a specific certificate.
    In this case, $\mathit{CombinedVerify}^{t + 1}(v', \Sigma') = \mathit{true}$.
    Hence, a correct process broadcasts a \textsc{help\_reply} message containing a (partial) signature of $v'$ (line~\ref{line:send_help_reply}).
    However, this is impossible as all correct processes propose the same value $v \neq v'$.
    Thus, this case is impossible, as well.
    
    \item Let $\Sigma'$ be a general certificate.
    Therefore, $\mathit{CombinedVerify}^{t + 1}(\text{``any value''}, \Sigma') = \mathit{true}$.
    Hence, a correct process $P$ has broadcast an \textsc{allow-any} message (line~\ref{line:broadcast_allow_any}).
    Thus, $P$ has not obtained a certificate by the beginning of round 3 (due to the check at line~\ref{line:check_for_broadcast_allow_any}).
    However, this contradicts \Cref{lemma:by_round_3}, implying that this case cannot occur.
\end{compactitem}
As no case is possible, there does not exist a certificate $\Sigma'$ for $v'$.
Thus, the lemma.
\end{proof}

Finally, we are ready to prove the correctness of \name.

\begin{theorem}
\name (\Cref{algorithm:strong_new}) is correct.
\end{theorem}
\begin{proof}
Termination of \name follows from (1) the fact that each correct process eventually proposes to closed-box Byzantine agreement (at line~\ref{line:propose_to_adaptive}), and (2) termination of to closed-box Byzantine agreement.
Similarly, agreement of \name follows directly from agreement of closed-box Byzantine agreement.
Finally, strong validity of \name follows from \Cref{lemma:strong_validity}.
\end{proof}

\paragraph{Proof of complexity.}
We start by showing that, if $f \leq t_{\mathit{opt}}$ faults, no correct process sends more than $f$ messages from round 1 onward.

\begin{lemma} \label{lemma:f_messages}
If $f \leq t_{\mathit{opt}}$, no correct process sends more than $f$ messages from round 1 onward.
\end{lemma}
\begin{proof}
Let us fix any correct process $P$.
If $f \leq t_{\mathit{opt}}$, $P$ obtains a fast certificate (at line~\ref{line:fast_certificate_obtained}) before starting round 1 (by the liveness property of \textsc{bucket}).
Hence, after the attainment of the fast certificate, $P$ can only send $\textsc{help\_reply}$ messages in round 2 (line~\ref{line:send_help_reply}).
As no correct process ever broadcasts a \textsc{help\_req} message (line~\ref{line:broadcast_help_req}), $P$ sends (at most) $f$ \textsc{help\_reply} messages (line~\ref{line:send_help_reply}).
This, the lemma.
\end{proof}

Next, we show that no correct process sends more than $n$ messages from round 1 onward.

\begin{lemma} \label{lemma:n_messages}
No correct process sends more than $n$ messages from round 1 onward.
\end{lemma}
\begin{proof}
Follows directly from \Cref{algorithm:strong_new}.
\end{proof}

Finally, we are ready to prove the communication complexity of \name.

\begin{theorem}
\name (\Cref{algorithm:strong_new}) has $O(n \cdot f)$ communication complexity.
\end{theorem}
\begin{proof}
We consider two cases:
\begin{compactitem}
    \item Let $f \leq t_{\mathit{opt}}$.
    In this case, correct processes send $O(n \cdot f)$ words before round 1, i.e., during $t_{\mathit{opt}} + 1$ ``rounds'' of \textsc{bucket}. \pierre{I still do not know how to prove this statement in a compact manner. A rigorous prove would probably mention $\cert^{+}$ and a result like (poorly written) lemma \ref{lemma:bucket+_efficiency}} 
    From round 1 onward, each correct process sends at most $f$ messages (by \Cref{lemma:f_messages}), each with a single word.
    Finally, as the communication complexity of closed-box Byzantine agreement is $O(n \cdot f)$, the overall communication complexity is $O(n \cdot f)$ in this case.
    
    \item Otherwise, $f \in O(n)$.
    Recall that $t_{\mathit{opt}} \in O(n)$.
    Before round 1, correct processes send (at most) $O(n^2)$ words.
    Moreover, from round 1 onward, each correct process sends at most $n$ messages (by \Cref{lemma:n_messages}), each with a single words.
    Lastly, in closed-box Byzantine agreement, correct processes exchange (at most) $O(n^2)$ words.
    Thus, in this case, the communication complexity of \name is $O(n^2)$, which is $O(n \cdot f)$ as $f \in O(n)$.
\end{compactitem}
As the communication complexity of \name is $O(n \cdot f)$ in both cases, the theorem holds.
\end{proof}
